# Supplementary material for: HandOccNet: Occlusion-Robust 3D Hand Mesh Estimation Network
Source: arXiv:2203.14564 source file (2022-03-28)
Supplement: Supplementary file 1 [file fit.tex]

\begin{table*}[t]
    \centering
    \begin{tabular}{c|c|c|c|c|c}
        \toprule
        Input & Output &  layer & kernel & stride & output shape\\
        \midrule
        $\mathbf{F}_{\text{S}}$ & - & - & - & - & $256 \times 32 \times 32$ \\
        $\mathbf{F}_{\text{P}}$ & - & - & - & - & $256 \times 32 \times 32$ \\
        \midrule
        $q_{\text{soft}}$ & $\mathbf{F}_{\text{S}}$ & conv & $1 \times 1$ & 1 & $256 \times 32 \times 32$\\
        $q_{\text{sig}}$ & $\mathbf{F}_{\text{S}}$ & conv & $1 \times 1$ & 1 & $256 \times 32 \times 32$\\
        $k_{\text{soft}}$ & $\mathbf{F}_{\text{P}}$ & conv & $1 \times 1$ & 1 & $256 \times 32 \times 32$\\
        $k_{\text{sig}}$ & $\mathbf{F}_{\text{P}}$ & conv & $1 \times 1$ & 1 & $256 \times 32 \times 32$\\
        $k_{\text{sig}}$ & $\mathbf{F}_{\text{P}}$ & conv & $1 \times 1$ & 1 & $256 \times 32 \times 32$\\
        $v$ & $\mathbf{F}_{\text{P}}$ & conv & $1 \times 1$ & 1 & $256 \times 32 \times 32$\\
        \midrule
        $q_{\text{soft}}$ & $q_{\text{soft}}$ & reshape & - & - & $32*32  \times 256$\\
        $q_{\text{sig}}$ & $q_{\text{sig}}$ & reshape & - & - & $32*32  \times 256$\\
        $k_{\text{soft}}$ & $k_{\text{soft}}$ & reshape & - & - & $32*32  \times 256$\\
        $k_{\text{sig}}$ & $k_{\text{sig}}$ & reshape & - & - & $32*32  \times 256$\\
        $k_{\text{sig}}$ & $k_{\text{sig}}$ & reshape & - & - & $32*32  \times 256$\\
        $v$ & $v$ & reshape & - & - & $32*32  \times 256$\\
        \midrule
        $q_{\text{soft}}$ $\And$ $k_{\text{soft}}$ & - & Matrix mult. & - & - & $32*32 \times 32*32$\\
        - & $\mathbf{C}_{\text{soft}}$ & softmax & - & - & $32*32 \times 32*32$\\
        \midrule
        $q_{\text{sig}}$ $\And$ $k_{\text{sig}}$ & - & Matrix mult. & - & - & $32*32 \times 32*32$\\
        - & - & average pooling & - & - & $32*32 \times 1$\\
        - & - & FC & - & - & $32*32 \times 1$\\
        - & $\mathbf{C}_{\text{sig}}$ & sigmoid & - & - & $32*32 \times 1$\\
        \midrule
        $\mathbf{C}_{\text{soft}}$ $\And$ $\mathbf{C}_{\text{sig}}$ & $\mathbf{C}$ & Element mult. & - & - & $32*32 \times 32*32$\\
        \midrule
        $\mathbf{C}_{\text{soft}}$ $\And$ $v$ & $\mathbf{R}_{\text{FIT}}$ & Matrix mult. & - & - & $32*32 \times 256$\\
        \midrule
        $\mathbf{R}_{\text{FIT}}$ & - & FC & - & - & $32*32 \times 256$\\
        - & - & ReLU & - & - & $32*32 \times 256$\\
        - & - & FC & - & - & $32*32 \times 256$\\
        - & - & Dropout & - & - & $32*32 \times 256$\\
        - & - & Connections & - & - & $32*32 \times 256$\\
        - & $\mathbf{F}_{\text{FIT}}$ & reshape & - & - & $256 \times 32 \times 32$\\
        \bottomrule
    \end{tabular}
    \tabcspace
    \caption{FIT architecture details.}
    \label{sup_tab:fit}
    \tabcspace
\end{table*}
