# Supplementary material for: HandOccNet: Occlusion-Robust 3D Hand Mesh Estimation Network
Source: arXiv:2203.14564 source file (2022-03-28)
Supplement: Supplementary file 2 [file model_figure.tex]

\begin{figure}[t]
    \centering

    \newcommand{\hhp}{\hspace{0.05\linewidth}}
    \subfloat[The overall architecure of HandOccNet, which consists of backbone, FIT, SET, and regressor.\label{sup_fig:model}]{
    \includegraphics[width=0.98\linewidth]{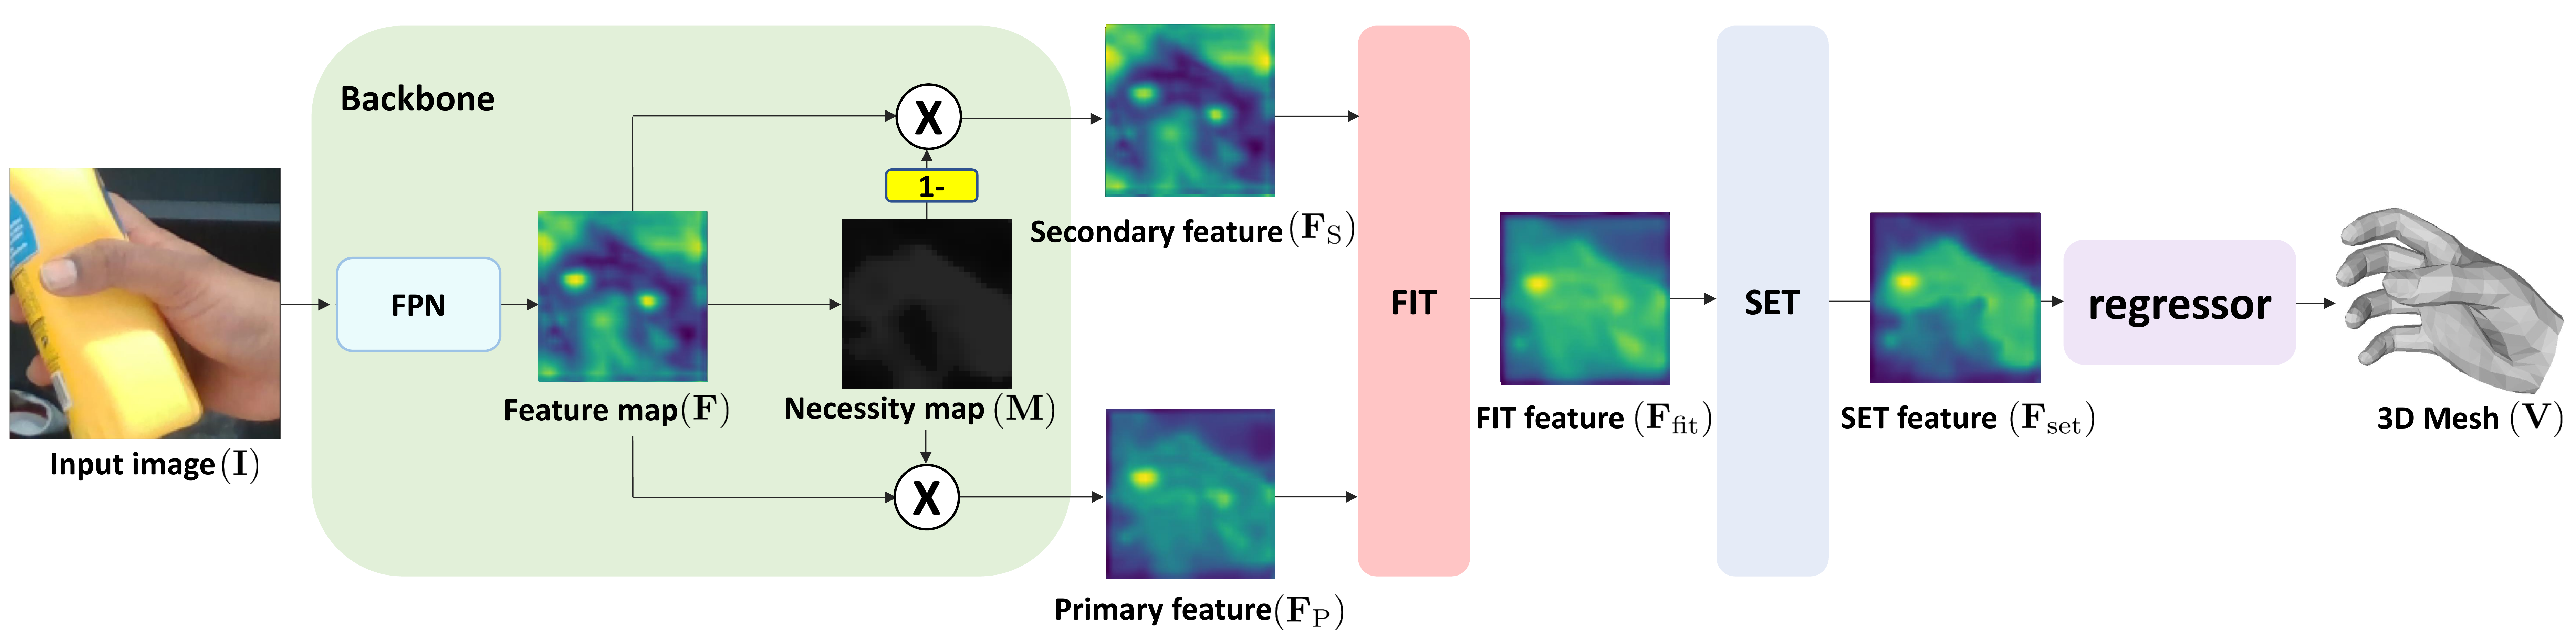}
    }
    \\
    \vspace{3mm}
    \subfloat[The overall pipeline of FIT. \label{sup_fig:fit}]{
    \includegraphics[height=0.22\linewidth]{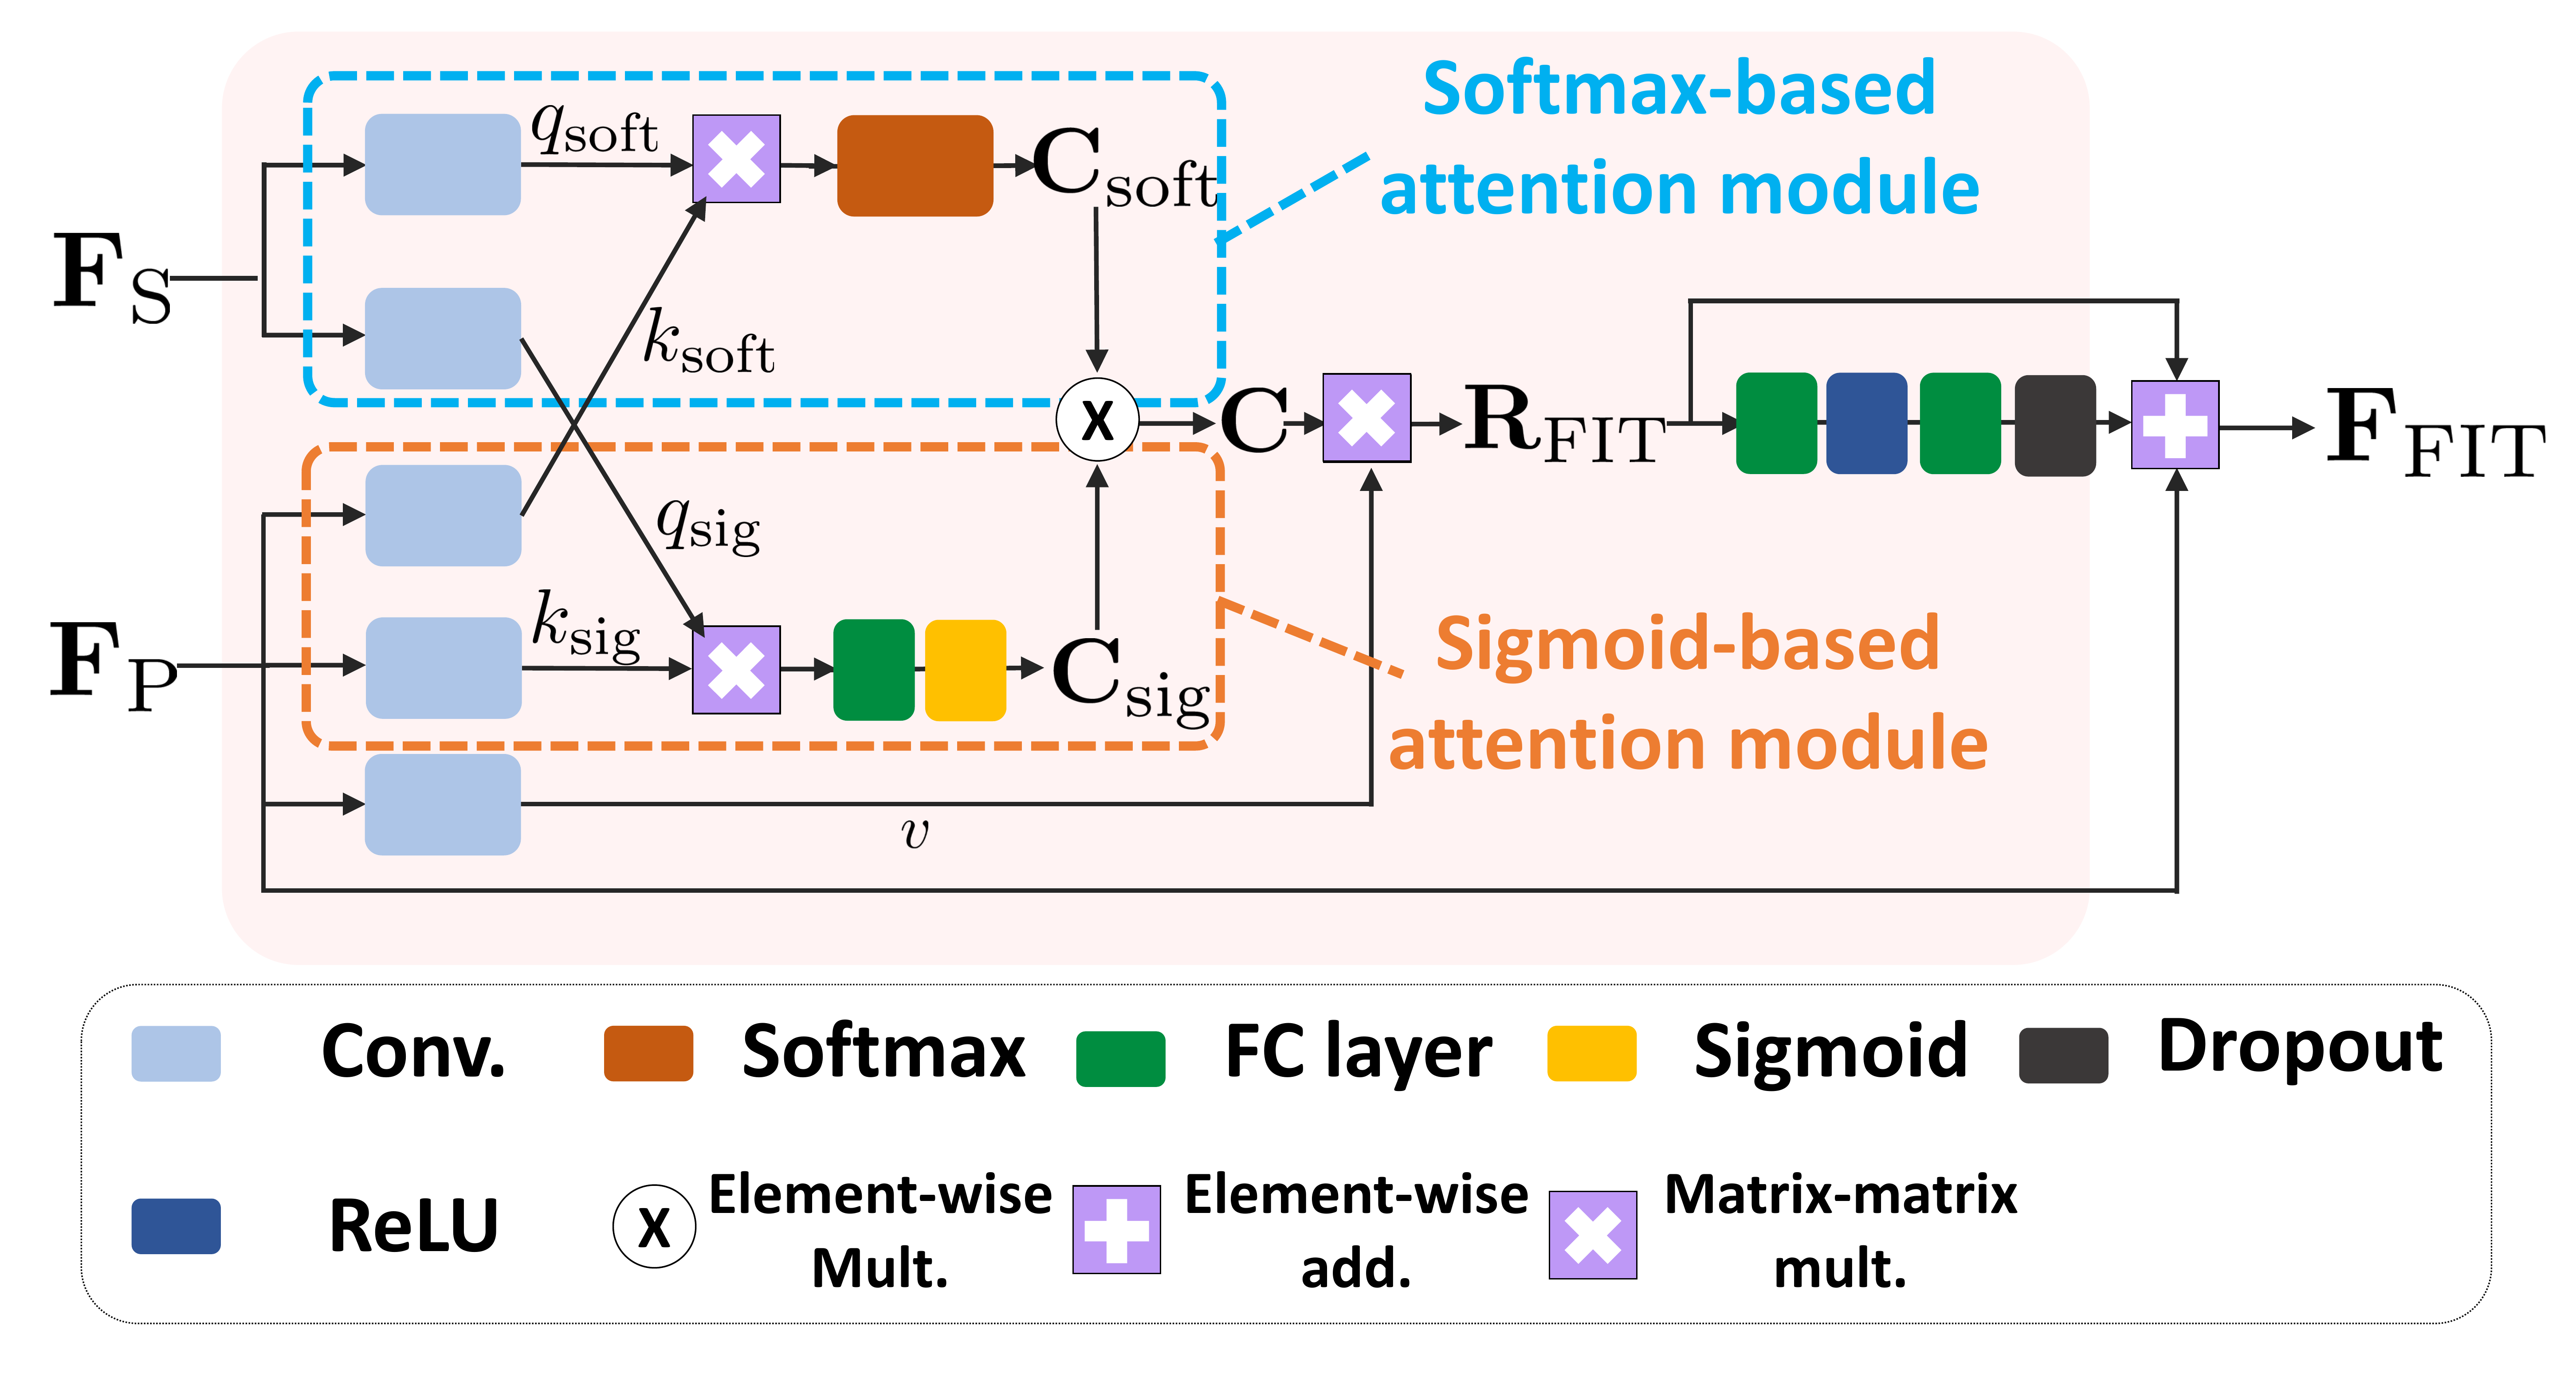}
    }
    \hhp
    \subfloat[The overall pipeline of SET. \label{sup_fig:set}]{
    \includegraphics[height=0.22\linewidth]{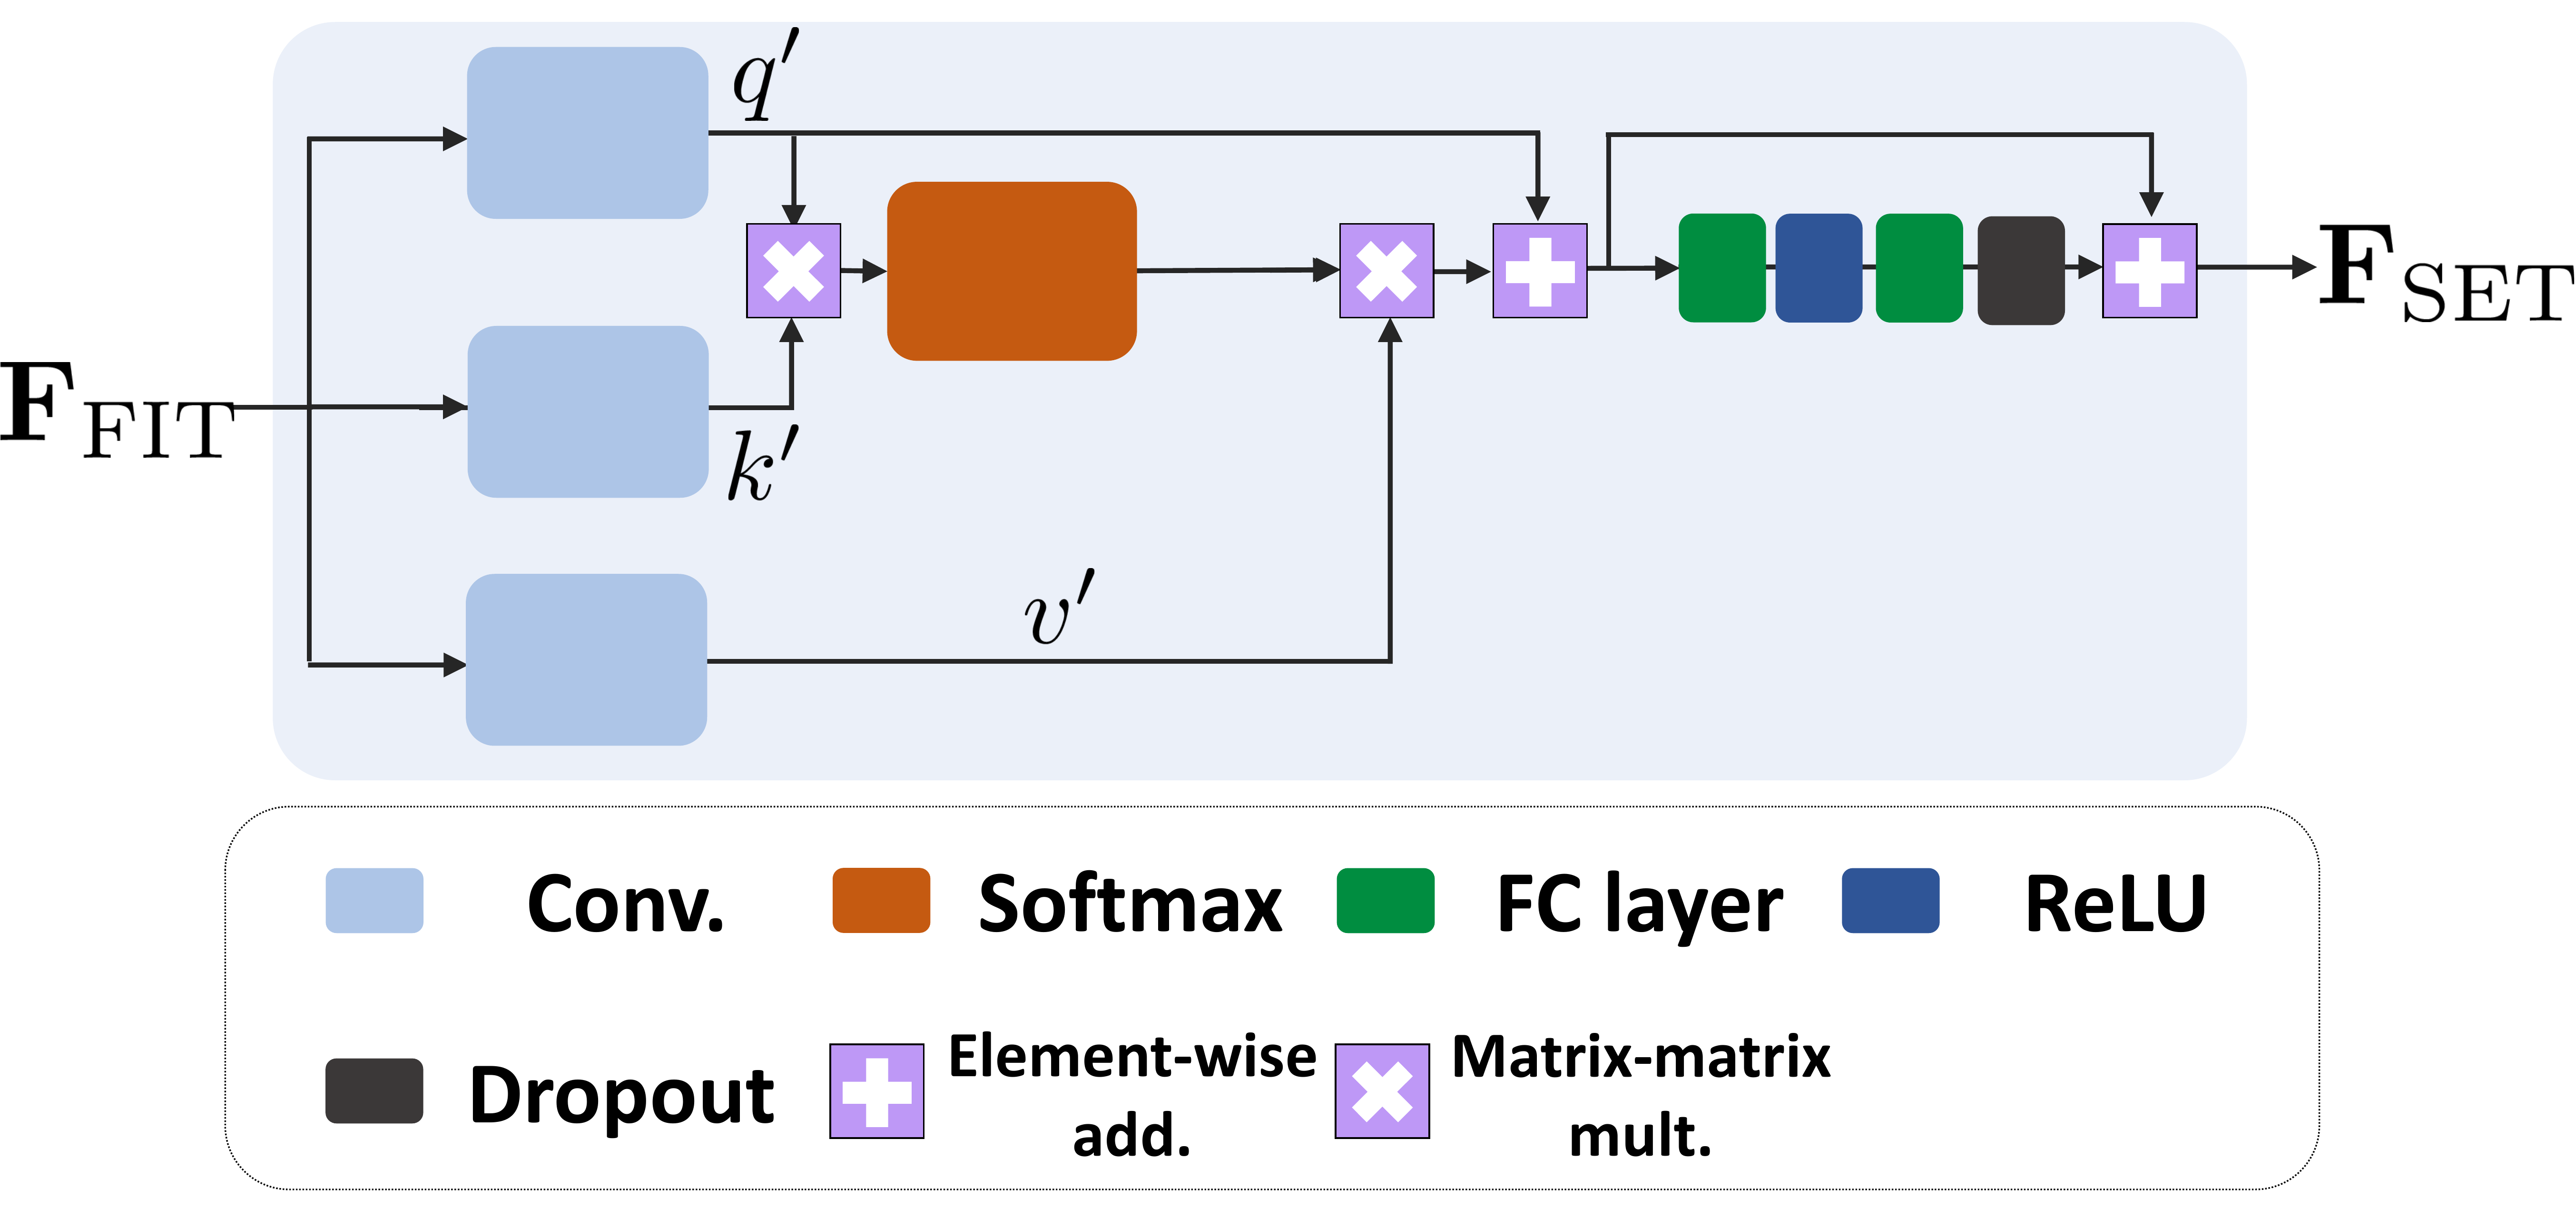}
    }
    \figcspace
    \caption{\textbf{Overall architecture and components of our HandOccNet.}}
    \label{fig:model}
    \figspace
\end{figure}
